# Supplementary material for: A General Framework For Detecting Anomalous Inputs to DNN Classifiers
Source: arXiv:2007.15147 source file (2021-06-17)
Supplement: Supplementary file 1 [file test_statistics_additional.tex]

\section{Test Statistics at the DNN Layers}
\label{sec:test_stats_appendix}
In section \S~\ref{sec:test_statistics}, we briefly described the multinomial test statistic which is based on class counts from the $k$-nearest neighbors (kNN) of a DNN layer representation. Here we provide a detailed and formal description of the multinomial test statistic. To demonstrate the generality of the proposed method, we present three additional test statistics that are also based on local statistical properties calculated from the kNN of a DNN layer representation.
For this discussion, we define the following additional terms. Recall that $\,D_a = \{(\bfx^{(0)}_n, \cdots, \bfx^{(L)}_n, c_n, \hat{c}_n), ~n \in [N]\}\,$ is a set of labeled samples augmented with the DNN layer representations and the predicted class.
Let 
\[
\mathcal{X}^{(\ell)}_c = \{\bfx^{(\ell)}_n, ~n \in [N] \,:\, c_n = c\}, ~~c \in [m]
\]
define the set of representations from layer $\ell$ corresponding to labeled samples from class $c$. Similarly, let 
\[
\widetilde{\mathcal{X}}^{(\ell)}_c = \{\bfx^{(\ell)}_n, ~n \in [N] \,:\, \hat{c}_n = c\}, ~~c \in [m]
\]
define the set of representations from layer $\ell$ corresponding to the samples predicted into class $c$. The index set of the $k$-nearest neighbors of a layer representation $\,\bfx^{(\ell)} \in \reals^{d_\ell}\,$ relative to the dataset $\,\mathcal{D}_a\,$ is denoted by $\,N^{(\ell)}_k(\bfx^{(\ell)}, \mathcal{D}_a) \,\subset\, [N]\,$. For brevity, we drop $\,\mathcal{D}_a\,$ from the notation.

\smallskip
\noindent{\bf Multinomial class count based test statistic}

If we consider a set of natural inputs to the DNN that are predicted into a class $\hat{c}$, the distribution of class counts from the kNN of its layer representations may be expected to follow a certain distribution that has a higher probability for class $\hat{c}$ than the rest. This observation can also be applied to the natural inputs from a given true class $c$. Let $\,(k^{(\ell)}_1, \cdots, k^{(\ell)}_m)\,$ denote the tuple of class counts from the kNN $\,N^{(\ell)}_k(\bfx^{(\ell)})\,$ of a layer representation $\bfx^{(\ell)}$ such that $\,k^{(\ell)}_i \in \lbrace0, 1, \cdots, k\rbrace\,$ and $\,\sum_{i} k^{(\ell)}_i = k$. The natural or null distribution of the kNN class counts at a layer $\ell$ conditioned on a predicted class $\hat{c}$ can be captured by the following multinomial distribution
\begin{equation}\label{eq:multinom}
p(k^{(\ell)}_1, \cdots, k^{(\ell)}_m \cond \widehat{C}=\hat{c}) ~=~ k! \,\myprod_{i=1}^m \frac{[\pi^{(\ell)}_{i \cond \hat{c}}]^{k^{(\ell)}_i}}{k^{(\ell)}_i!},
\end{equation}
%\vspace{-0.03in}
where $\,(\pi^{(\ell)}_{1 \cond \hat{c}}, \cdots, \pi^{(\ell)}_{m \cond \hat{c}})\,$ are multinomial probability parameters (specific to class $\hat{c}$ and layer $\ell$) that are constrained to lie in the $\,m - 1$ probability simplex $\,\Delta_m$. These parameters, although unknown, can be estimated from the labeled subset of $\,\mathcal{D}_a\,$ predicted into class $\,\hat{c}$, $\,\{(\bfx^{(0)}_n, \cdots, \bfx^{(L)}_n, c_n, \hat{c}_n), ~n = 1, \cdots, N \,:\, \hat{c}_n = \hat{c}\}\,$, using the framework of maximum likelihood or maximum-a-posteriori (MAP) estimation. We use MAP estimation with the Dirichlet conjugate prior distribution~\cite{barber2012} and hyper-parameters (a prior count from each class) set to a small nonzero value in order to avoid $0$ estimates for the probability parameters.

If a test input $\bfx$ classified into class $\hat{c}$ by the DNN follows the natural data distribution, we would expect distribution Eq. (\ref{eq:multinom}) to be a good fit for the class counts observed from its kNN at layer $\ell$. A well-known goodness-of-fit test for the multinomial distribution is the likelihood ratio test (LRT), which computes a log likelihood ratio as the test statistic~\cite{read2012goodness}. In order to test whether the observed class counts $\,(k^{(\ell)}_1, \cdots, k^{(\ell)}_m)\,$ from layer $\ell$, given predicted class $\hat{c}$, is consistent with distribution (\ref{eq:multinom}), the LRT test statistic is given by
\vspace{-0.07in}
\begin{equation}\label{eq:test_stat_lrt_pred}
T_p(\bfx^{(\ell)}, \hat{c}) ~= \mysum_{i=1}^m \,k^{(\ell)}_i \,\log\frac{k^{(\ell)}_i}{k \,\pi^{(\ell)}_{i \cond \hat{c}}}.
\end{equation}
This statistic is non-negative, with larger values corresponding to a larger deviation from the null distribution (\ref{eq:multinom}).

In a similar way, the natural or null distribution of the kNN class counts at a layer $\ell$ conditioned on a true class $c$ can be captured by the following multinomial distribution
\begin{equation}\label{eq:multinom_true}
p(k^{(\ell)}_1, \cdots, k^{(\ell)}_m \cond C = c) ~=~ k! \,\myprod_{i=1}^m \frac{[\widetilde{\pi}^{(\ell)}_{i \cond c}]^{k^{(\ell)}_i}}{k^{(\ell)}_i!}.
\end{equation}
The LRT test statistic corresponding to this multinomial distribution is given by
\begin{equation}
\label{eq:test_stat_lrt_true}
T_s(\bfx^{(\ell)}, c) ~= \mysum_{i=1}^m \,k^{(\ell)}_i \,\log\frac{k^{(\ell)}_i}{k \,\widetilde{\pi}^{(\ell)}_{i \cond c}}.
\end{equation}
Since the true class of a test input is unknown, we calculate this test statistic for each candidate true class $\,c \in [m]$. 
Although we use the LRT test statistic as a class count deviation measure, we do not rely on its asymptotic properties such as convergence to the $\chi^2$ distribution (when scaled by the factor $-2$), which would not be applicable in our scenario where $k$ is a small integer.

\smallskip
\noindent{\bf Binomial class count based test statistic}

This is a specialization of the multinomial test statistic, wherein instead of focusing on the kNN counts from all classes, we focus on the kNN count from a particular class (either the predicted class or a candidate true class). Consider an input $\bfx$ with layer representations $\,\bfx^{(\ell)}, ~~\ell = 0, 1, \cdots, L\,$ and predicted class $\hat{c}$. Let $\,k^{(\ell)}_{\hat{c}} \in \{0, 1, \cdots, k\}\,$ be the number of $k$-nearest neighbors from class $\hat{c}$ for the representation $\bfx^{(\ell)}$ from layer $\ell$. This count can be interpreted as the number of successes $\,k^{(\ell)}_{\hat{c}}\,$ in a binomial distribution with $k$ trials. We define the binomial test statistic given a class $c$ as the proportion of $k$-nearest neighbors that are not from the same class $c$. The test statistics at layer $\ell$ conditioned on the predicted class $\hat{c}$ and on each candidate true class are defined respectively as,
\beqa
\label{eq:test_stat_binom}
T_p(\bfx^{(\ell)}, \hat{c}) &=& \frac{k \,-\, k^{(\ell)}_{\hat{c}}}{k}, \nonumber \\
T_s(\bfx^{(\ell)}, c) &=& \frac{k \,-\, k^{(\ell)}_c}{k}, ~~\forall c \in [m].
\eeqa
The test statistics are bounded in $\,[0, 1]\,$ and measure the non-conformity of the class labels among the k-nearest neighbors of a layer representation, with larger values corresponding to a larger non-conformity. We note the similarity of this test statistic with the non-conformity score computed by the deep KNN method~\cite{papernot2018deep}, with a key difference that deep KNN calculates a single non-conformity score (per class) by summing the non-conforming class counts across the layers.

%\medskip
\newpage
\noindent{\bf Trust Score based test statistic}

The trust score was proposed by \cite{jiang2018trust} as a confidence score for a classifier that indicates when the classifier's prediction on a test input is likely to be correct. We first provide an informal definition of the $\alpha$-high density set $\,H_{\alpha}(f)\,$ for $\,\alpha \in [0, 1]\,$ and a continuous density function $f$ as -- the set of all points with density larger than a certain value $\lambda^{}_{\alpha}$ such that $\,1 - \alpha\,$ fraction of the probability mass is contained in $\,H_{\alpha}(f)\,$ (refer to \cite{jiang2018trust} for the formal definition). Given a set of points $\,\mathcal{X}_c\,$ from each class $\,c \in [m]$, the trust score estimates the $\alpha$-high density set $\,\widehat{H}_{\alpha}(f_c)\,$ for each class-conditional density $\,f_c, ~c \in [m]\,$ using the kNN distances of points from $\,\mathcal{X}_c$. For the special case of $\,\alpha = 0\,$ the density level-set estimate reduces to the set of all points from class $c$, \ie $\,\widehat{H}_{0}(f_c) = \mathcal{X}_c$. 

Given a test input $\bfx$ that is predicted into class $\hat{c}$ by the classifier, the trust score associated with the classifier's prediction on $\bfx$ is defined as~\cite{jiang2018trust}
\vspace{-0.05in}
\begin{equation*}
\xi(\bfx, \hat{c}) ~=~ \frac{\displaystyle\min_{i \,\in\, [m] \setminus \{\hat{c}\}} d_{\textrm{haus}}(\bfx, \widehat{H}_{\alpha}(f_i))}{d_{\textrm{haus}}(\bfx, \widehat{H}_{\alpha}(f_{\hat{c}}))},
\end{equation*}
where $d_{\textrm{haus}}$ is the Hausdorff distance, which in this case reduces to the nearest neighbor distance $\,d_{\textrm{haus}}(\bfx, \mathcal{X}) \,=\, \min_{\bfy \in \mathcal{X}} d(\bfx, \bfy)$ between a point $\bfx$ and set $\mathcal{X}$. In other words, the trust score is the ratio of the minimum distance from a point to the $\alpha$-high density set of a class different from the predicted class, to the distance from a point to the $\alpha$-high density set of the predicted class. The score is non-negative and unbounded above, with larger values indicating a higher level of trust or confidence in the classifier's prediction. 

For an input $\bfx$ with representation $\,\bfx^{(\ell)}\,$ at layer $\ell$ and predicted class $\hat{c}$, we define the test statistic conditioned on the predicted class as the inverse of the trust score
\begin{equation}
T_p(\bfx^{(\ell)}, \hat{c}) ~=~ \frac{ d_{\textrm{haus}}(\bfx^{(\ell)}, \widetilde{\mathcal{X}}^{(\ell)}_{\hat{c}}) }{ \displaystyle\min_{i \,\in\, [m] \setminus \{\hat{c}\}} d_{\textrm{haus}}(\bfx^{(\ell)}, \widetilde{\mathcal{X}}^{(\ell)}_i) }
\end{equation}
so that an anomalous input (with a low trust score) will have a large test statistic value. Note that we use the special case of the trust score with $\,\alpha = 0\,$ for simplicity. The set $\,\widetilde{\mathcal{X}}^{(\ell)}_{\hat{c}}\,$ is a representative sample of layer representations from the class-conditional density given the predicted class $\,\widehat{C} = \hat{c}$. Similarly, the test statistics at layer $\ell$ conditioned on each candidate true class are defined as
%\vspace{-0.07in}
\begin{equation}
T_s(\bfx^{(\ell)}, c) ~=~ \frac{ d_{\textrm{haus}}(\bfx^{(\ell)}, \mathcal{X}^{(\ell)}_c) }{ \displaystyle\min_{i \,\in\, [m] \setminus \{c\}} d_{\textrm{haus}}(\bfx^{(\ell)}, \mathcal{X}^{(\ell)}_i) }, ~~\forall c \in [m].
\end{equation}
In this case, the set $\,\mathcal{X}^{(\ell)}_c\,$ is a representative sample of layer representations from the class-conditional density given the true class $\,C = c$.

\smallskip
\noindent{\bf Local Intrinsic Dimensionality based test statistic}

Local intrinsic dimensionality (LID) at a point provides an indication of the dimension of the sub-manifold containing the point that would best fit the distribution of data in a local neighborhood of that point~\cite{carter2009local, ansuini2019intrinsic}. 
%In broader terms, LID can be understood as a measure of the rate of growth of the number of data points as the distance from a reference point increases.
For a formal definition of LID in terms of the cumulative distribution function of the distance from a point to other points from the same distribution, the reader is referred to prior works~\cite{ma2018characterizing_iclr, amsaleg2015estimating}. In practice, LID is estimated from the distances of a point to its k-nearest neighbors using ideas from extreme value theory. We use the maximum likelihood estimator (MLE) of LID from \cite{amsaleg2015estimating} that is also used in the work of \cite{ma2018characterizing_iclr} to estimate the LID of DNN layer representations. Consider a point $\bfx$ whose distances to its k-nearest neighbors from a set of points $\mathcal{X}$ are denoted by $\,r_i(\bfx, \mathcal{X}), ~i = 1, \cdots, k$. The MLE estimate of LID from \cite{amsaleg2015estimating} is given by
\vspace{-0.07in}
\begin{equation*}
\widehat{\textrm{LID}}(\bfx, \mathcal{X}) ~=~ -\left(\frac{1}{k} \mysum_{i=1}^k \,\log\frac{r_i(\bfx, \mathcal{X})}{r_k(\bfx, \mathcal{X})} \right)^{-1}.
\end{equation*}

For an input $\bfx$ with representation $\,\bfx^{(\ell)}\,$ at layer $\ell$ and predicted class $\hat{c}$, we define the test statistics based on LID conditioned on the predicted class $\hat{c}$ and on each candidate true class as
\beqa
T_p(\bfx^{(\ell)}, \hat{c}) &=& \widehat{\textrm{LID}}(\bfx^{(\ell)}, \mathcal{X}^{(\ell)}_{\hat{c}}), \nonumber \\
T_s(\bfx^{(\ell)}, c) &=& \widehat{\textrm{LID}}(\bfx^{(\ell)}, \mathcal{X}^{(\ell)}_c), ~~\forall c \in [m].
\eeqa
We expect anomalous inputs to the DNN to produce test statistics (LID) that are larger than that observed on natural inputs, as observed by \cite{ma2018characterizing_iclr} on adversarial inputs. 

\smallskip
\noindent{\bf Combining Multiple Test Statistics.}

We note that it is straightforward to include more than one test statistic per-layer in the framework of \proposed. For example, the multinomial, binomial, and trust score based test statistics could be calculated at each layer, resulting in a test statistic vector of length $3\,(L + 1)$. With this change, the method for estimating p-values from the test statistics, either combined or multivariate, and the scoring function for adversarial and OOD detection do not require any modifications. Combining multiple test statistics in this way could be an approach to improving the detection rate of \proposed, with a modest increase in the computation. It may also be argued that it is harder for a defense-aware adaptive attacker to generate adversarial samples that can evade a detector based on multiple test statistics at the DNN layers.

In Appendix~\ref{app:performance_test_stats}, we provide results comparing the performance of \proposed with the test statistics defined here on the adversarial detection task.
